# Supplementary material for: A New Matrix Truncation Method for Improving Approximate Factorisation Preconditioners
Source: arXiv:2312.06417 source file (2024-10-09)
Supplement: Supplementary file 1 [file appendix.tex]

\section{Additional results for large matrices}\label{appendix:large:nys=0}

Randomised linear algebra was used to produce the results in 
\cref{table:GHS_psdef_crankseg_1,table:gyro_m,table:Dubcova1,table:GHS_psdef_apache1,table:Rothberg_cfd1,table:Schmid_thermal1}. Specifically, the Nyström approximation was
used to compute $\BregTruncPositive{\tilde E}$. To isolate the effect of this choice, we show
the results for the same matrices and parameters, but where we have employed the Krylov--Schur
method discussed in \cref{sec:Bregman_directions:smallest} to estimate all the eigenvalues
of the approximation $\BregTruncPositive{\tilde E}$ used in \cref{eq:Bregman_preconditioner:approx}.
The results are shown in \cref{table:GHS_psdef_crankseg_1:nonys,table:gyro_m:nonys,table:Dubcova1:nonys,table:GHS_psdef_apache1:nonys,table:Rothberg_cfd1:nonys,table:Schmid_thermal1:nonys}, with minor improvements to number of PCG iterations for
$\alpha > 0$.

{
\begin{table}%[h!]%[tbhp]
\scriptsize
\caption{Results for \texttt{GHS/psdef\_crankseg\_1}.}\label{table:GHS_psdef_crankseg_1:nonys}
\begin{center}
\begin{tabular*}{0.73\textwidth}{l @{\extracolsep{\fill}} *{8}{c}}
\toprule 
Preconditioner & $r$ & $\alpha$ & Rel. residual & Iteration count & Construction ($s$) & Solve ($s$) & Matvecs\\
\midrule
\input{csvs/large/nys=0/GHS_psdef_crankseg_1_ichol_type=nofill_droptol=0_diagcomp=0_nnzS=10614210_nnzQ=5333507.csv}
\\[-\normalbaselineskip]\bottomrule
\end{tabular*}
\end{center}
\end{table}
}

{
\begin{table}%[h!]%[tbhp]
\scriptsize
\caption{Results for \texttt{Oberwolfach/gyro\_m}.}\label{table:gyro_m:nonys}
\begin{center}
\begin{tabular*}{0.73\textwidth}{l @{\extracolsep{\fill}} *{8}{c}}
\toprule 
Preconditioner & $r$ & $\alpha$ & Rel. residual & Iteration count & Construction ($s$) & Solve ($s$) & Matvecs\\
\midrule
\input{csvs/large/nys=0/Oberwolfach_gyro_m_ichol_type=nofill_droptol=0_diagcomp=0_nnzS=340431_nnzQ=178896.csv}
\\[-\normalbaselineskip]\bottomrule
\end{tabular*}
\end{center}
\end{table}
}

{
\begin{table}%[h!]%[tbhp]
\scriptsize
\caption{Results for \texttt{UTEP/Dubcova1}.}\label{table:Dubcova1:nonys}
\begin{center}
\begin{tabular*}{0.73\textwidth}{l @{\extracolsep{\fill}} *{8}{c}}
\toprule 
Preconditioner & $r$ & $\alpha$ & Rel. residual & Iteration count & Construction ($s$) & Solve ($s$) & Matvecs\\
\midrule
\input{csvs/large/nys=0/UTEP_Dubcova1_ichol_type=nofill_droptol=0_diagcomp=0_nnzS=253009_nnzQ=134569.csv}
\\[-\normalbaselineskip]\bottomrule
\end{tabular*}
\end{center}
\end{table}
}

{
\begin{table}%[h!]%[tbhp]
\scriptsize
\caption{Results for \texttt{GHS/psdef\_apache1.}}\label{table:GHS_psdef_apache1:nonys}
\begin{center}
\begin{tabular*}{0.73\textwidth}{l @{\extracolsep{\fill}} *{8}{c}}
\toprule 
Preconditioner & $r$ & $\alpha$ & Rel. residual & Iteration count & Construction ($s$) & Solve ($s$) & Matvecs\\
\midrule
\input{csvs/large/nys=0/GHS_psdef_apache1_ichol_type=nofill_droptol=0_diagcomp=0_nnzS=542184_nnzQ=311492.csv}
\\[-\normalbaselineskip]\bottomrule
\end{tabular*}
\end{center}
\end{table}
}

{
\begin{table}%[h!]%[tbhp]
\scriptsize
\caption{Results for \texttt{Rothberg/cfd1}.}\label{table:Rothberg_cfd1:nonys}
\begin{center}
\begin{tabular*}{0.73\textwidth}{l @{\extracolsep{\fill}} *{8}{c}}
\toprule 
Preconditioner & $r$ & $\alpha$ & Rel. residual & Iteration count & Construction ($s$) & Solve ($s$) & Matvecs\\
\midrule
\input{csvs/large/nys=0/Rothberg_cfd1_ichol_type=nofill_droptol=0_diagcomp=0_nnzS=1825580_nnzQ=948118.csv}
\\[-\normalbaselineskip]\bottomrule
\end{tabular*}
\end{center}
\end{table}
}

{
\begin{table}%[h!]%[tbhp]
\scriptsize
\caption{Results for \texttt{Schmid/thermal1.}}\label{table:Schmid_thermal1:nonys}
\begin{center}
\begin{tabular*}{0.73\textwidth}{l @{\extracolsep{\fill}} *{8}{c}}
\toprule 
Preconditioner & $r$ & $\alpha$ & Rel. residual & Iteration count & Construction ($s$) & Solve ($s$) & Matvecs\\
\midrule
\input{csvs/large/nys=0/Schmid_thermal1_ichol_type=nofill_droptol=0_diagcomp=0_nnzS=574458_nnzQ=328556.csv}
\\[-\normalbaselineskip]\bottomrule
\end{tabular*}
\end{center}
\end{table}
}
